# Supplementary material for: Nuclear energy density optimization: Shell structure
Source: arXiv:1312.1746 source file (2014-04-28)
Supplement: Supplementary file 1 [file unedf_supp_mk2_NS.pdf]

**Supplemental material for: Nuclear energy density optimization: Shell structure**

M. Kortelainen,[1, 2, 3] J. McDonnell,[2, 3, 4] W. Nazarewicz,[2, 3, 5] E. Olsen,[2] P.-G. Reinhard,[6] J. Sarich,[7] N. Schunck,[4, 2, 3] S. M. Wild,[7] D. Davesne,[8] J. Erler,[9] and A. Pastore[10]

[1] *Department of Physics, University of Jyväskylä, P.O. Box 35 (YFL), FI-40014 Finland*
[2] *Department of Physics and Astronomy, University of Tennessee, Knoxville, TN 37996, USA*
[3] *Physics Division, Oak Ridge National Laboratory, Oak Ridge, TN 37831, USA*
[4] *Physics Division, Lawrence Livermore National Laboratory, Livermore, CA 94551, USA*
[5] *Institute of Theoretical Physics, Warsaw University, ul. Ho˙ za 69, PL-00681, Warsaw, Poland*
[6] *Institut für Theoretische Physik, Universität Erlangen, D-91054 Erlangen, Germany*
[7] *Mathematics and Computer Science Division, Argonne National Laboratory, Argonne, IL 60439, USA*
[8] *Université de Lyon, F-69622 Lyon, France; Université de Lyon 1, Villeurbanne; CNRS/IN2P3, Institut de Physique Nucléaire de Lyon*
[9] *Division Biophysics of Macromolecules, German Cancer Research Center (DKFZ), Im Neuenheimer Feld 580, D-69120 Heidelberg, Germany*
[10] *Institut d'Astronomie et d'Astrophysique, Université Libre de Bruxelles - CP226, 1050 Brussels, Belgium*

## I. REMARKS

1. The definition of the coupling constants and their relations to nuclear matter observables can be found in Phys. Rev. C **82**, 024313 (2010), Eqs.(2), (3), (17), (18), (19), (20), (30), (31), (32). Note that in Eq.(2), the tensor term was written under the implicit assumption of conserved parity. The actual tensor term implemented in our DFT solvers HFBTHO and HFODD reads, for channel *t = 0, 1*

$$\mathcal{H}_{\rm tens} = C_t^{JJ} \sum_{\mu\nu} J_{\nu,t} J_{\mu\nu,t} = \frac{1}{3} C_t^{JJ} \left(J_t^0\right)^2 + \frac{1}{2} C_t^{JJ} \boldsymbol{J}_t^2 + C_t^{JJ} \mathbb{J}_t^2 \qquad (1)$$

with the pseudoscalar, vector and pseudotensor terms defined as usual

$$J_t^{(0)} = \sum_{\mu} J_{\mu\mu,t}, \quad \boldsymbol{J}_{\kappa,t} = \sum_{\mu\nu} \epsilon_{\kappa\mu\nu} J_{\mu\nu,t}, \quad \mathbb{J}_{\mu\nu,t} = \frac{1}{2}\left(J_{\mu\nu,t} + J_{\nu\mu,t}\right) - \delta_{\mu\nu} \frac{1}{3} J_t^{(0)}. \qquad (2)$$

The coupling constants $C^{JJ}$ given below correspond to the definition (1).

2. Most of the atomic masses used in the fit of UNEDF functionals were extracted from the 2003 Atomic Mass Data evaluation of Nucl. Phys. A **729**, 337 (2003). These masses were updated with data from JYFLTRAP, available at: http://research.jyu.fi/igisol/JYFLTRAP_masses/gs_masses.txt. In the case where two different masses $M_i$ with uncertainties $\delta M_i$ were available for the same nucleus, the actual mass was deduced from the formula

$$M = \frac{\omega_1 M_1 + \omega_2 M_2}{\omega_1 + \omega_2} \qquad \delta M = \frac{1}{\sqrt{\omega_1 + \omega_2}}$$

with

$$\omega_i = \frac{1}{\delta M_i^2}$$

3. Table II in Phys. Rev. C **82**, 024313 (2010) erroneously lists masses of spherical nuclei as obtained from the 1995 Atomic Mass Data Evaluation instead of the 2003 version. The Table XI below gives the correct masses.

4. The physical constants used to define the kinetic energy and Coulomb potential are: $\hbar^2/2m$ = 20.73553 MeV, $e^2$ = 1.439978408596513.

## II. UNEDF PARAMETRIZATIONS

### A. Hybrid Nuclear Matter - Coupling Constants Representation

TABLE I: UNEDF0.

| Parameter | Value |
|---|---|
| $\rho_c$ | 0.1605260000000000 |
| $E^{NM}/A$ | -16.0559000000000000 |
| $K^{NM}$ | 230.0000000000000000 |
| $a_{sym}{}^{NM}$ | 30.5429000000000000 |
| $L_{sym}{}^{NM}$ | 45.0804000000000000 |
| $1/M_s{}^*$ | 0.9000000000000000 |
| $1/M_v{}^*$ | 1.2498380000000000 |
| $C_0{}^{\rho\Delta\rho}$ | -55.2606000000000000 |
| $C_1{}^{\rho\Delta\rho}$ | -55.6226000000000000 |
| $C_0{}^{\rho\nabla J}$ | -79.5308000000000000 |
| $C_1{}^{\rho\nabla J}$ | 45.6302000000000000 |
| $C_0{}^{JJ}$ | 0.0000000000000000 |
| $C_1{}^{JJ}$ | 0.0000000000000000 |
| Center of Mass | True |
| $V_0{}^n$ | -170.3740000000000000 |
| $V_0{}^p$ | -199.2020000000000000 |

TABLE II: UNEDF1.

| Parameter | Value |
|---|---|
| $\rho_c$ | 0.1587067693325870 |
| $E^{NM}/A$ | -15.8000000000000000 |
| $K^{NM}$ | 220.0000000000000000 |
| $a_{sym}{}^{NM}$ | 28.9867890577721000 |
| $L_{sym}{}^{NM}$ | 40.0047904804136000 |
| $1/M_s{}^*$ | 0.9924233322833640 |
| $1/M_v{}^*$ | 1.2498385742322700 |
| $C_0{}^{\rho\Delta\rho}$ | -45.1351310222373030 |
| $C_1{}^{\rho\Delta\rho}$ | -145.3821679080570000 |
| $C_0{}^{\rho\nabla J}$ | -74.0263331764599000 |
| $C_1{}^{\rho\nabla J}$ | -35.6582611147917000 |
| $C_0{}^{JJ}$ | 0.0000000000000000 |
| $C_1{}^{JJ}$ | 0.0000000000000000 |
| Center of Mass | False |
| $V_0{}^n$ | -186.0653995751240000 |
| $V_0{}^p$ | -206.5795938901060000 |

TABLE III: UNEDF2.

| Parameter | Value |
|---|---|
| $\rho_c$ | 0.1563106221970741 |
| $E^{NM}/A$ | -15.8000000000000000 |
| $K^{NM}$ | 239.9295680224370528 |
| $a_{sym}{}^{NM}$ | 29.1310064707736984 |
| $L_{sym}{}^{NM}$ | 40.0000000000000000 |
| $1/M_s{}^*$ | 1.0737638041479800 |
| $1/M_v{}^*$ | 1.2498385742322700 |
| $C_0{}^{\rho\Delta\rho}$ | -46.8314091470605973 |
| $C_1{}^{\rho\Delta\rho}$ | -113.1637907952590040 |
| $C_0{}^{\rho\nabla J}$ | -64.3088624157838069 |
| $C_1{}^{\rho\nabla J}$ | -38.6501946851355029 |
| $C_0{}^{JJ}$ | -54.4333635973721002 |
| $C_1{}^{JJ}$ | -65.9030310445938028 |
| Center of Mass | False |
| $V_0{}^n$ | -208.8890019625710000 |
| $V_0{}^p$ | -230.3299840386279980 |

### B. Full Coupling Constants Representation

TABLE IV: UNEDF0.

| Parameter | Value |
|---|---|
| $C_0^{\rho 2}$ | -706.382928878428856000 |
| $C_1^{\rho 2}$ | 240.049520427681131000 |
| $C_{0D}^{\rho 2}$ | 868.871771539645351000 |
| $C_{1D}^{\rho 2}$ | -69.051895748163161700 |
| $C_0^{\rho\tau}$ | -12.917240820801611200 |
| $C_1^{\rho\tau}$ | -45.189416942675947600 |
| $\gamma$ | 0.321955989588264435 |
| $C_0^{\rho\Delta\rho}$ | -55.260600000000000000 |
| $C_1^{\rho\Delta\rho}$ | -55.622600000000000000 |
| $C_0^{\rho\nabla J}$ | -79.530800000000000000 |
| $C_1^{\rho\nabla J}$ | 45.630200000000000000 |
| $C_0^{JJ}$ | 0.000000000000000000 |
| $C_1^{JJ}$ | 0.000000000000000000 |
| Center of Mass | True |
| $V_0^n$ | -170.374000000000000000 |
| $V_0^p$ | -199.202000000000000000 |

TABLE V: UNEDF1.

| Parameter | Value |
|---|---|
| $C_0^{\rho 2}$ | -779.373008720865300000 |
| $C_1^{\rho 2}$ | 287.722131583286796000 |
| $C_{0D}^{\rho 2}$ | 891.477890442349690000 |
| $C_{1D}^{\rho 2}$ | -200.587774317884879000 |
| $C_0^{\rho\tau}$ | -0.989915057807676746 |
| $C_1^{\rho\tau}$ | -33.632097070183554900 |
| $\gamma$ | 0.270018011502707600 |
| $C_0^{\rho\Delta\rho}$ | -45.135131022237303000 |
| $C_1^{\rho\Delta\rho}$ | -145.382167908057000000 |
| $C_0^{\rho\nabla J}$ | -74.026333176459900000 |
| $C_1^{\rho\nabla J}$ | -35.658261114791700000 |
| $C_0^{JJ}$ | 0.000000000000000000 |
| $C_1^{JJ}$ | 0.000000000000000000 |
| Center of Mass | False |
| $V_0^n$ | -186.065399575123990000 |
| $V_0^p$ | -206.579593890105997000 |

TABLE VI: UNEDF2.

| Parameter | Value |
|---|---|
| $C_0^{\rho 2}$ | -650.796319465688839000 |
| $C_1^{\rho 2}$ | 291.664014339185485000 |
| $C_{0D}^{\rho 2}$ | 768.327705882033570000 |
| $C_{1D}^{\rho 2}$ | -283.187292227492492000 |
| $C_0^{\rho\tau}$ | 9.785205588243096390 |
| $C_1^{\rho\tau}$ | -23.357361297703533900 |
| $\gamma$ | 0.351455132555483607 |
| $C_0^{\rho\Delta\rho}$ | -46.831409147060597300 |
| $C_1^{\rho\Delta\rho}$ | -113.163790795259004000 |
| $C_0^{\rho\nabla J}$ | -64.308862415783806900 |
| $C_1^{\rho\nabla J}$ | -38.650194685135502900 |
| $C_0^{JJ}$ | -54.433363597372100200 |
| $C_1^{JJ}$ | -65.903031044593802800 |
| Center of Mass | False |
| $V_0^n$ | -208.88900196257100100 |
| $V_0^p$ | -230.32998403862799800 |

## III. UNEDF DATASETS

### A. UNEDF0

TABLE X: Masses of deformed nuclei.

| Number | Z | N | Energy (MeV) | Weight (MeV) |
|---|---|---|---|---|
| 1 | 108 | 156 | -1925.69700 | 2.0 |
| 2 | 106 | 154 | -1908.03775 | 2.0 |
| 3 | 104 | 152 | -1889.70921 | 2.0 |
| 4 | 102 | 154 | -1897.72867 | 2.0 |
| 5 | 102 | 152 | -1884.68553 | 2.0 |
| 6 | 102 | 150 | -1870.38620 | 2.0 |
| 7 | 100 | 156 | -1901.67298 | 2.0 |
| 8 | 100 | 154 | -1890.11218 | 2.0 |
| 9 | 100 | 152 | -1878.05634 | 2.0 |
| 10 | 100 | 150 | -1864.65753 | 2.0 |
| 11 | 100 | 148 | -1850.68221 | 2.0 |
| 12 | 100 | 146 | -1836.30537 | 2.0 |
| 13 | 98 | 156 | -1891.28115 | 2.0 |
| 14 | 98 | 154 | -1880.44518 | 2.0 |
| 15 | 98 | 152 | -1869.16473 | 2.0 |
| 16 | 98 | 150 | -1856.95416 | 2.0 |
| 17 | 98 | 148 | -1843.95952 | 2.0 |
| 18 | 98 | 146 | -1830.42944 | 2.0 |
| 19 | 98 | 144 | -1816.42832 | 2.0 |
| 20 | 96 | 150 | -1847.03719 | 2.0 |
| 21 | 96 | 148 | -1835.05913 | 2.0 |
| 22 | 96 | 144 | -1809.50224 | 2.0 |
| 23 | 94 | 144 | -1800.52348 | 2.0 |
| 24 | 92 | 144 | -1789.70112 | 2.0 |
| 25 | 92 | 142 | -1777.85822 | 2.0 |
| 26 | 90 | 142 | -1766.01478 | 2.0 |
| 27 | 72 | 104 | -1418.40662 | 2.0 |
| 28 | 70 | 108 | -1431.26039 | 2.0 |
| 29 | 70 | 100 | -1377.76048 | 2.0 |
| 30 | 68 | 104 | -1391.21286 | 2.0 |
| 31 | 68 | 102 | -1378.69547 | 2.0 |
| 32 | 66 | 102 | -1362.59073 | 2.0 |
| 33 | 66 | 100 | -1350.47410 | 2.0 |
| 34 | 66 | 98 | -1337.71449 | 2.0 |
| 35 | 66 | 96 | -1323.78552 | 2.0 |
| 36 | 66 | 94 | -1309.13406 | 2.0 |
| 37 | 66 | 92 | -1293.72542 | 2.0 |
| 38 | 66 | 90 | -1277.70063 | 2.0 |
| 39 | 64 | 98 | -1321.47330 | 2.0 |
| 40 | 64 | 96 | -1308.99194 | 2.0 |
| 41 | 64 | 94 | -1295.59749 | 2.0 |
| 42 | 64 | 92 | -1281.30023 | 2.0 |
| 43 | 64 | 90 | -1266.32864 | 2.0 |
| 44 | 64 | 88 | -1251.18707 | 2.0 |

TABLE XI: Masses of spherical nuclei.

| Number | Z | N | Energy (MeV) | Weight (MeV) |
|---|---|---|---|---|
| 45 | 82 | 132 | -1662.75325 | 2.0 |
| 46 | 82 | 130 | -1653.97679 | 2.0 |
| 47 | 82 | 128 | -1645.01508 | 2.0 |
| 48 | 82 | 126 | -1635.89266 | 2.0 |
| 49 | 82 | 124 | -1621.78701 | 2.0 |
| 50 | 82 | 122 | -1606.96857 | 2.0 |
| 51 | 82 | 120 | -1591.64987 | 2.0 |
| 52 | 82 | 118 | -1575.81684 | 2.0 |
| 53 | 82 | 116 | -1559.48128 | 2.0 |
| 54 | 50 | 74 | -1049.79795 | 2.0 |
| 55 | 50 | 72 | -1035.36456 | 2.0 |
| 56 | 50 | 70 | -1020.38103 | 2.0 |
| 57 | 50 | 68 | -1004.78946 | 2.0 |
| 58 | 50 | 66 | -988.51881 | 2.0 |
| 59 | 50 | 64 | -971.40893 | 2.0 |
| 60 | 50 | 62 | -953.36675 | 2.0 |
| 61 | 50 | 58 | -914.50074 | 2.0 |
| 62 | 28 | 36 | -561.71668 | 2.0 |
| 63 | 28 | 34 | -545.22083 | 2.0 |
| 64 | 28 | 32 | -526.80421 | 2.0 |
| 65 | 28 | 30 | -506.41717 | 2.0 |
| 66 | 28 | 28 | -483.95050 | 2.0 |
| 67 | 20 | 30 | -427.47131 | 2.0 |
| 68 | 20 | 28 | -415.97198 | 2.0 |
| 69 | 20 | 26 | -398.75027 | 2.0 |
| 70 | 20 | 24 | -380.94104 | 2.0 |
| 71 | 20 | 22 | -361.87704 | 2.0 |
| 72 | 20 | 20 | -342.03360 | 2.0 |

TABLE XII: R.m.s. radii of spherical nuclei.

| Number | Z | N | Radius (fm) | Weight (fm) |
|---|---|---|---|---|

| | | | | |
|---|---|---|---|---|
| 73 | 82 | 132 | 5.50638 | 0.02 |
| 74 | 82 | 130 | 5.48896 | 0.02 |
| 75 | 82 | 128 | 5.46952 | 0.02 |
| 76 | 82 | 126 | 5.45007 | 0.02 |
| 77 | 82 | 124 | 5.43971 | 0.02 |
| 78 | 82 | 122 | 5.42834 | 0.02 |
| 79 | 82 | 120 | 5.41899 | 0.02 |
| 80 | 82 | 118 | 5.40357 | 0.02 |
| 81 | 82 | 116 | 5.39422 | 0.02 |
| 82 | 50 | 74 | 4.60966 | 0.02 |
| 83 | 50 | 72 | 4.59800 | 0.02 |
| 84 | 50 | 70 | 4.58634 | 0.02 |
| 85 | 50 | 68 | 4.57366 | 0.02 |
| 86 | 50 | 66 | 4.55895 | 0.02 |
| 87 | 50 | 64 | 4.54220 | 0.02 |
| 88 | 50 | 62 | 4.52748 | 0.02 |
| 89 | 50 | 58 | 4.49294 | 0.02 |
| 90 | 28 | 36 | 3.78703 | 0.02 |
| 91 | 28 | 34 | 3.76550 | 0.02 |
| 92 | 28 | 32 | 3.73372 | 0.02 |
| 93 | 28 | 30 | 3.68964 | 0.02 |
| 94 | 28 | 28 | 3.66189 | 0.02 |
| 95 | 20 | 30 | 3.43752 | 0.02 |
| 96 | 20 | 28 | 3.39070 | 0.02 |
| 97 | 20 | 26 | 3.41260 | 0.02 |
| 98 | 20 | 24 | 3.43245 | 0.02 |
| 99 | 20 | 22 | 3.42049 | 0.02 |
| 100 | 20 | 20 | 3.38282 | 0.02 |

TABLE XIII: Odd-even mass difference $\Delta^{(3)}$ for protons and neutron.

| Number | Z | N | $\Delta^{(3)}$ (MeV) | Weight (MeV) | Nucl. |
|---|---|---|---|---|---|
| 101 | 100 | 152 | 0.5148145 | 0.05 | n |
| 102 | 92 | 144 | 0.5691325 | 0.05 | n |
| 103 | 72 | 104 | 0.6747180 | 0.05 | n |
| 104 | 66 | 98 | 0.6786245 | 0.05 | n |
| 105 | 96 | 148 | 0.5661460 | 0.05 | p |
| 106 | 92 | 142 | 0.6061590 | 0.05 | p |
| 107 | 68 | 102 | 0.5040435 | 0.05 | p |
| 108 | 66 | 94 | 0.7278535 | 0.05 | p |

### B. UNEDF1

TABLE XIV: Masses of deformed nuclei.

| Number | Z | N | Energy (MeV) | Weight (MeV) |
|---|---|---|---|---|
| 1 | 108 | 156 | -1925.69700 | 2.0 |
| 2 | 106 | 154 | -1908.03775 | 2.0 |
| 3 | 104 | 152 | -1889.70921 | 2.0 |
| 4 | 102 | 154 | -1897.72867 | 2.0 |
| 5 | 102 | 152 | -1884.68553 | 2.0 |
| 6 | 102 | 150 | -1870.38620 | 2.0 |
| 7 | 100 | 156 | -1901.67298 | 2.0 |
| 8 | 100 | 154 | -1890.11218 | 2.0 |
| 9 | 100 | 152 | -1878.05634 | 2.0 |
| 10 | 100 | 150 | -1864.65753 | 2.0 |
| 11 | 100 | 148 | -1850.68221 | 2.0 |
| 12 | 100 | 146 | -1836.30537 | 2.0 |
| 13 | 98 | 156 | -1891.28115 | 2.0 |
| 14 | 98 | 154 | -1880.44518 | 2.0 |
| 15 | 98 | 152 | -1869.16473 | 2.0 |
| 16 | 98 | 150 | -1856.95416 | 2.0 |
| 17 | 98 | 148 | -1843.95952 | 2.0 |
| 18 | 98 | 146 | -1830.42944 | 2.0 |
| 19 | 98 | 144 | -1816.42832 | 2.0 |
| 20 | 96 | 150 | -1847.03719 | 2.0 |
| 21 | 96 | 148 | -1835.05913 | 2.0 |
| 22 | 96 | 146 | -1822.56507 | 2.0 |
| 23 | 96 | 144 | -1809.50224 | 2.0 |
| 24 | 94 | 146 | -1812.70387 | 2.0 |
| 25 | 94 | 144 | -1800.52348 | 2.0 |
| 26 | 92 | 146 | -1800.98110 | 2.0 |
| 27 | 92 | 144 | -1789.70112 | 2.0 |
| 28 | 92 | 142 | -1777.85822 | 2.0 |
| 29 | 90 | 142 | -1766.01478 | 2.0 |
| 30 | 72 | 104 | -1418.40662 | 2.0 |
| 31 | 70 | 108 | -1431.26039 | 2.0 |
| 32 | 70 | 100 | -1377.76048 | 2.0 |
| 33 | 68 | 104 | -1391.21286 | 2.0 |
| 34 | 68 | 102 | -1378.69547 | 2.0 |
| 35 | 66 | 102 | -1362.59073 | 2.0 |
| 36 | 66 | 100 | -1350.47410 | 2.0 |
| 37 | 66 | 98 | -1337.71449 | 2.0 |

| | | | | |
|---|---|---|---|---|
| 38 | 66 | 96 | -1323.78552 | 2.0 |
| 39 | 66 | 94 | -1309.13406 | 2.0 |
| 40 | 66 | 92 | -1293.72542 | 2.0 |
| 41 | 66 | 90 | -1277.70063 | 2.0 |
| 42 | 64 | 98 | -1321.47330 | 2.0 |
| 43 | 64 | 96 | -1308.99194 | 2.0 |
| 44 | 64 | 94 | -1295.59749 | 2.0 |
| 45 | 64 | 92 | -1281.30023 | 2.0 |
| 46 | 64 | 90 | -1266.32864 | 2.0 |
| 47 | 64 | 88 | -1251.18707 | 2.0 |

TABLE XV: Masses of spherical nuclei.

| Number | Z | N | Energy (MeV) | Weight (MeV) |
|---|---|---|---|---|
| 48 | 82 | 132 | -1662.75325 | 2.0 |
| 49 | 82 | 130 | -1653.97679 | 2.0 |
| 50 | 82 | 128 | -1645.01508 | 2.0 |
| 51 | 82 | 126 | -1635.89266 | 2.0 |
| 52 | 82 | 124 | -1621.78701 | 2.0 |
| 53 | 82 | 122 | -1606.96857 | 2.0 |
| 54 | 82 | 120 | -1591.64987 | 2.0 |
| 55 | 82 | 118 | -1575.81684 | 2.0 |
| 56 | 82 | 116 | -1559.48128 | 2.0 |
| 57 | 50 | 74 | -1049.79795 | 2.0 |
| 58 | 50 | 72 | -1035.36456 | 2.0 |
| 59 | 50 | 70 | -1020.38103 | 2.0 |
| 60 | 50 | 68 | -1004.78946 | 2.0 |
| 61 | 50 | 66 | -988.51881 | 2.0 |
| 62 | 50 | 64 | -971.40893 | 2.0 |
| 63 | 50 | 62 | -953.36675 | 2.0 |
| 64 | 50 | 58 | -914.50074 | 2.0 |
| 65 | 28 | 36 | -561.71668 | 2.0 |
| 66 | 28 | 34 | -545.22083 | 2.0 |
| 67 | 28 | 32 | -526.80421 | 2.0 |
| 68 | 28 | 30 | -506.41717 | 2.0 |
| 69 | 28 | 28 | -483.95050 | 2.0 |
| 70 | 20 | 30 | -427.47131 | 2.0 |
| 71 | 20 | 28 | -415.97198 | 2.0 |
| 72 | 20 | 26 | -398.75027 | 2.0 |
| 73 | 20 | 24 | -380.94104 | 2.0 |
| 74 | 20 | 22 | -361.87704 | 2.0 |
| 75 | 20 | 20 | -342.03360 | 2.0 |

TABLE XVI: R.m.s. radii of spherical nuclei.

| Number | Z | N | Radius (fm) | Weight (fm) |
|---|---|---|---|---|
| 76 | 82 | 132 | 5.50638 | 0.02 |
| 77 | 82 | 130 | 5.48896 | 0.02 |
| 78 | 82 | 128 | 5.46952 | 0.02 |
| 79 | 82 | 126 | 5.45007 | 0.02 |
| 80 | 82 | 124 | 5.43971 | 0.02 |
| 81 | 82 | 122 | 5.42834 | 0.02 |
| 82 | 82 | 120 | 5.41899 | 0.02 |
| 83 | 82 | 118 | 5.40357 | 0.02 |
| 84 | 82 | 116 | 5.39422 | 0.02 |
| 85 | 50 | 74 | 4.60966 | 0.02 |
| 86 | 50 | 72 | 4.59800 | 0.02 |
| 87 | 50 | 70 | 4.58634 | 0.02 |
| 88 | 50 | 68 | 4.57366 | 0.02 |
| 89 | 50 | 66 | 4.55895 | 0.02 |
| 90 | 50 | 64 | 4.54220 | 0.02 |
| 91 | 50 | 62 | 4.52748 | 0.02 |
| 92 | 50 | 58 | 4.49294 | 0.02 |
| 93 | 28 | 36 | 3.78703 | 0.02 |
| 94 | 28 | 34 | 3.76550 | 0.02 |
| 95 | 28 | 32 | 3.73372 | 0.02 |
| 96 | 28 | 30 | 3.68964 | 0.02 |
| 97 | 28 | 28 | 3.66189 | 0.02 |
| 98 | 20 | 30 | 3.43752 | 0.02 |
| 99 | 20 | 28 | 3.39070 | 0.02 |
| 100 | 20 | 26 | 3.41260 | 0.02 |
| 101 | 20 | 24 | 3.43245 | 0.02 |
| 102 | 20 | 22 | 3.42049 | 0.02 |
| 103 | 20 | 20 | 3.38282 | 0.02 |

TABLE XVII: Odd-even mass difference $\Delta^{(3)}$ for protons and neutron.

| Number | Z | N | $\Delta^{(3)}$ (MeV) | Weight (MeV) | Nucl. |
|---|---|---|---|---|---|
| 104 | 100 | 152 | 0.5148145 | 0.05 | n |
| 105 | 92 | 144 | 0.5691325 | 0.05 | n |
| 106 | 72 | 104 | 0.6747180 | 0.05 | n |
| 107 | 66 | 98 | 0.6786245 | 0.05 | n |
| 108 | 96 | 148 | 0.5661460 | 0.05 | p |
| 109 | 92 | 142 | 0.6061590 | 0.05 | p |
| 110 | 68 | 102 | 0.5040435 | 0.05 | p |
| 111 | 66 | 94 | 0.7278535 | 0.05 | p |

TABLE XVIII: Excitation energy of fission isomer.

| Number | Z | N | $E^*_{SD}$ (MeV) | Weight (MeV) |
|---|---|---|---|---|
| 112 | 92 | 144 | 2.750 | 0.5 |
| 113 | 92 | 146 | 2.557 | 0.5 |
| 114 | 94 | 146 | 2.800 | 0.5 |
| 115 | 96 | 146 | 1.900 | 0.5 |

## C. UNEDF2

TABLE XIX: Masses of deformed nuclei.

| Number | Z | N | Energy (MeV) | Weight (MeV) |
|---|---|---|---|---|
| 1 | 108 | 156 | -1925.69700 | 2.0 |
| 2 | 106 | 154 | -1908.03775 | 2.0 |
| 3 | 104 | 152 | -1889.70921 | 2.0 |
| 4 | 102 | 154 | -1897.72867 | 2.0 |
| 5 | 102 | 152 | -1884.68553 | 2.0 |
| 6 | 102 | 150 | -1870.38620 | 2.0 |
| 7 | 100 | 156 | -1901.67298 | 2.0 |
| 8 | 100 | 154 | -1890.11218 | 2.0 |
| 9 | 100 | 152 | -1878.05634 | 2.0 |
| 10 | 100 | 150 | -1864.65753 | 2.0 |
| 11 | 100 | 148 | -1850.68221 | 2.0 |
| 12 | 100 | 146 | -1836.30537 | 2.0 |
| 13 | 98 | 156 | -1891.28115 | 2.0 |
| 14 | 98 | 154 | -1880.44518 | 2.0 |
| 15 | 98 | 152 | -1869.16473 | 2.0 |
| 16 | 98 | 150 | -1856.95416 | 2.0 |
| 17 | 98 | 148 | -1843.95952 | 2.0 |
| 18 | 98 | 146 | -1830.42944 | 2.0 |
| 19 | 98 | 144 | -1816.42832 | 2.0 |
| 20 | 96 | 150 | -1847.03719 | 2.0 |
| 21 | 96 | 148 | -1835.05913 | 2.0 |
| 22 | 96 | 146 | -1822.56507 | 2.0 |
| 23 | 96 | 144 | -1809.50224 | 2.0 |
| 24 | 94 | 146 | -1812.70387 | 2.0 |
| 25 | 94 | 144 | -1800.52348 | 2.0 |
| 26 | 92 | 146 | -1800.98110 | 2.0 |
| 27 | 92 | 144 | -1789.70112 | 2.0 |
| 28 | 92 | 142 | -1777.85822 | 2.0 |
| 29 | 90 | 142 | -1766.01478 | 2.0 |
| 30 | 72 | 104 | -1418.40662 | 2.0 |
| 31 | 70 | 108 | -1431.26039 | 2.0 |
| 32 | 70 | 100 | -1377.76048 | 2.0 |
| 33 | 68 | 104 | -1391.21286 | 2.0 |
| 34 | 68 | 102 | -1378.69547 | 2.0 |
| 35 | 66 | 102 | -1362.59073 | 2.0 |
| 36 | 66 | 100 | -1350.47410 | 2.0 |
| 37 | 66 | 98 | -1337.71449 | 2.0 |
| 38 | 66 | 96 | -1323.78552 | 2.0 |
| 39 | 66 | 94 | -1309.13406 | 2.0 |
| 40 | 66 | 92 | -1293.72542 | 2.0 |
| 41 | 66 | 90 | -1277.70063 | 2.0 |
| 42 | 64 | 98 | -1321.47330 | 2.0 |
| 43 | 64 | 96 | -1308.99194 | 2.0 |
| 44 | 64 | 94 | -1295.59749 | 2.0 |
| 45 | 64 | 92 | -1281.30023 | 2.0 |
| 46 | 64 | 90 | -1266.32864 | 2.0 |
| 47 | 64 | 88 | -1251.18707 | 2.0 |

TABLE XX: Masses of spherical nuclei.

| Number | Z | N | Energy (MeV) | Weight (MeV) |
|---|---|---|---|---|
| 48 | 82 | 132 | -1662.75325 | 2.0 |
| 49 | 82 | 130 | -1653.97679 | 2.0 |
| 50 | 82 | 128 | -1645.01508 | 2.0 |
| 51 | 82 | 126 | -1635.89266 | 2.0 |
| 52 | 82 | 124 | -1621.78701 | 2.0 |
| 53 | 82 | 122 | -1606.96857 | 2.0 |
| 54 | 82 | 120 | -1591.64987 | 2.0 |
| 55 | 82 | 118 | -1575.81684 | 2.0 |
| 56 | 82 | 116 | -1559.48128 | 2.0 |
| 57 | 50 | 82 | -1102.68603 | 2.0 |
| 58 | 50 | 74 | -1049.79795 | 2.0 |
| 59 | 50 | 72 | -1035.36456 | 2.0 |
| 60 | 50 | 70 | -1020.38103 | 2.0 |
| 61 | 50 | 68 | -1004.78946 | 2.0 |
| 62 | 50 | 66 | -988.51881 | 2.0 |
| 63 | 50 | 64 | -971.40893 | 2.0 |
| 64 | 50 | 62 | -953.36675 | 2.0 |
| 65 | 50 | 58 | -914.50074 | 2.0 |
| 66 | 28 | 36 | -561.71668 | 2.0 |
| 67 | 28 | 34 | -545.22083 | 2.0 |
| 68 | 28 | 32 | -526.80421 | 2.0 |

| | | | | |
|---|---|---|---|---|
| 69 | 28 | 30 | -506.41717 | 2.0 |
| 70 | 28 | 28 | -483.95050 | 2.0 |
| 71 | 20 | 30 | -427.47131 | 2.0 |
| 72 | 20 | 28 | -415.97198 | 2.0 |
| 73 | 20 | 26 | -398.75027 | 2.0 |
| 74 | 20 | 24 | -380.94104 | 2.0 |
| 75 | 20 | 22 | -361.87704 | 2.0 |
| 76 | 20 | 20 | -342.03360 | 2.0 |

TABLE XXI: R.m.s. radii of spherical nuclei.

| Number | Z | N | Radius (fm) | Weight (fm) |
|---|---|---|---|---|
| 77 | 82 | 132 | 5.50638 | 0.02 |
| 78 | 82 | 130 | 5.48896 | 0.02 |
| 79 | 82 | 128 | 5.46952 | 0.02 |
| 80 | 82 | 126 | 5.45007 | 0.02 |
| 81 | 82 | 124 | 5.43971 | 0.02 |
| 82 | 82 | 122 | 5.42834 | 0.02 |
| 83 | 82 | 120 | 5.41899 | 0.02 |
| 84 | 82 | 118 | 5.40357 | 0.02 |
| 85 | 82 | 116 | 5.39422 | 0.02 |
| 86 | 50 | 74 | 4.60966 | 0.02 |
| 87 | 50 | 72 | 4.59800 | 0.02 |
| 88 | 50 | 70 | 4.58634 | 0.02 |
| 89 | 50 | 68 | 4.57366 | 0.02 |
| 90 | 50 | 66 | 4.55895 | 0.02 |
| 91 | 50 | 64 | 4.54220 | 0.02 |
| 92 | 50 | 62 | 4.52748 | 0.02 |
| 93 | 50 | 58 | 4.49294 | 0.02 |
| 94 | 28 | 36 | 3.78703 | 0.02 |
| 95 | 28 | 34 | 3.76550 | 0.02 |
| 96 | 28 | 32 | 3.73372 | 0.02 |
| 97 | 28 | 30 | 3.68964 | 0.02 |
| 98 | 28 | 28 | 3.66189 | 0.02 |
| 99 | 20 | 30 | 3.43752 | 0.02 |
| 100 | 20 | 28 | 3.39070 | 0.02 |
| 101 | 20 | 26 | 3.41260 | 0.02 |
| 102 | 20 | 24 | 3.43245 | 0.02 |
| 103 | 20 | 22 | 3.42049 | 0.02 |
| 104 | 20 | 20 | 3.38282 | 0.02 |

TABLE XXII: Odd-even mass difference $\Delta^{(3)}$ for protons and neutron.

| Number | Z | N | $\Delta^{(3)}$ (MeV) | Weight (MeV) | Nucl. |
|---|---|---|---|---|---|
| 105 | 100 | 152 | 0.5148145 | 0.1 | n |
| 106 | 90 | 142 | 0.6814525 | 0.1 | n |
| 107 | 92 | 144 | 0.5691325 | 0.1 | n |
| 108 | 72 | 104 | 0.6747180 | 0.1 | n |
| 109 | 66 | 98 | 0.6786245 | 0.1 | n |
| 110 | 74 | 50 | 1.2504275 | 0.1 | n |
| 111 | 70 | 50 | 1.3168945 | 0.1 | n |
| 112 | 96 | 148 | 0.5661460 | 0.1 | p |
| 113 | 92 | 142 | 0.6061590 | 0.1 | p |
| 114 | 90 | 142 | 0.8132845 | 0.1 | p |
| 115 | 76 | 90 | 1.1690370 | 0.1 | p |
| 116 | 68 | 102 | 0.5040435 | 0.1 | p |
| 117 | 66 | 94 | 0.7278535 | 0.1 | p |

TABLE XXIII: Excitation energy of fission isomer.

| Number | Z | N | $E^*_{SD}$ (MeV) | Weight (MeV) |
|---|---|---|---|---|
| 118 | 92 | 144 | 2.750 | 0.5 |
| 119 | 92 | 146 | 2.557 | 0.5 |
| 120 | 94 | 146 | 2.800 | 0.5 |
| 121 | 96 | 146 | 1.900 | 0.5 |

TABLE XXIV: Single-particle splittings in spherical nuclei.

| Number | Z | N | Nucl. | Splitting | Value (MeV) | Weight (MeV) |
|---|---|---|---|---|---|---|
| 122 | 20 | 20 | n | $f_{5/2}-f_{7/2}$ | 6.80 | 1.2 |
| 123 | 20 | 20 | n | $f_{7/2}-d_{3/2}$ | 7.28 | 1.2 |
| 124 | 20 | 20 | p | $f_{7/2}-d_{3/2}$ | 7.24 | 1.2 |
| 125 | 20 | 28 | n | $f_{5/2}-f_{7/2}$ | 8.80 | 1.2 |
| 126 | 20 | 28 | p | $f_{5/2}-f_{7/2}$ | 4.92 | 1.2 |
| 127 | 50 | 82 | n | $h_{9/2}-h_{11/2}$ | 6.68 | 1.2 |
| 128 | 50 | 82 | p | $g_{7/2}-g_{9/2}$ | 6.03 | 1.2 |
| 129 | 82 | 126 | n | $i_{11/2}-i_{13/2}$ | 6.08 | 1.2 |
| 130 | 82 | 126 | p | $h_{9/2}-h_{11/2}$ | 5.56 | 1.2 |

TABLE XXV: Single-particle energies from binding energies and excitation energies of corresponding levels from ENSDF data.

| Number | Z | N | Nucl. | Splitting | Value (MeV) |
|---|---|---|---|---|---|
| 122 | 20 | 20 | n | $f_{5/2}-f_{7/2}$ | 2.58 |
| 123 | 20 | 20 | n | $f_{7/2}-d_{3/2}$ | 7.28 |
| 124 | 20 | 20 | p | $f_{7/2}-d_{3/2}$ | 7.25 |
| 125 | 20 | 28 | n | $f_{5/2}-f_{7/2}$ | 8.38 |
| 126 | 20 | 28 | p | $f_{5/2}-f_{7/2}$ | 4.07[1] |
| 127 | 50 | 82 | n | $h_{9/2}-h_{11/2}$ | 6.47 |
| 128 | 50 | 82 | p | $g_{7/2}-g_{9/2}$ | 6.03 |
| 129 | 82 | 126 | n | $i_{11/2}-i_{13/2}$ | 5.84 |
| 130 | 82 | 126 | p | $h_{9/2}-h_{11/2}$ | 5.55 |

1) This value is uncertain since there are also other levels with possible Jπ=5/2+ assignment.
